# Supplementary material for: Estimation and Inference in Factor Copula Models with Exogenous Covariates
Source: arXiv:2107.03366 source file (2022-12-01)
Supplement: Supplementary file 1 [file copula_ref_supp.tex]

					%\bibitem[\protect\citeauthoryear{Anderson and Rubin}{Anderson and Rubin}{1956}]{ar56}
		%Anderson, T.~W., and R.~Rubin (1956).
		%\newblock Statistical inference in factor analysis.
%\newblock {\em Proceedings of the Third Berkeley Symposium on Mathematical Statistics and Probability, 1954–1955,\/} {\em 5}, 111--150.  

					\bibitem[\protect\citeauthoryear{Akritas and Van Keilegom}{Akritas and Van Keilegom}{2001}]{avk01}
		Akritas, M.~G., and I.~Van Keilegom (2001).
		\newblock Non-parametric estimation of the residual distribution.
\newblock {\em Scandinavian Journal of Statistics\/} {\em 28}, 549--567. \doi{10.1111/1467-9469.00254}


					\bibitem[\protect\citeauthoryear{Andrews and Pollard}{Andrews and Pollard}{1994}]{anpo94}
		Andrews, D.~W.~K.,  and D. Pollard (1994).
		\newblock  An introduction to functional central limit theorems for dependent stochastic processes.
\newblock {\em International Statistical Review\/} {\em 62}, 119--132. \doi{10.2307/1403549}

					%\bibitem[\protect\citeauthoryear{Bae \textit{et al.}}{Bae \textit{et al.}}{2010}]{baetal10}
%Bae, J.-S., D.~Jun, and S. Levental(2010).
		%\newblock  The uniform CLT for martingale difference arrays under the uniformly ingegrable entropy.
%\newblock {\em  Bull. Korean Math. Soc.\/} {\em 47}, 39--51. \doi{10.4134/BKMS.2010.47.1.039.}

					%\bibitem[\protect\citeauthoryear{Baur and McDermott}{Baur and McDermott}{2010}]{Baurmc10}
		%Baur, D.~G., and T.~K. McDermott (2010).
		%\newblock  Is gold a safe haven? International evidence.
%\newblock {\em Journal of Banking \& Finance\/} {\em 34}, 1886--1898. \doi{10.1016/j.jbankfin.2009.12.008}

					\bibitem[\protect\citeauthoryear{Berghaus \textit{et al.}}{Berghaus \textit{et al.}}{2017}]{betal17}
		Berghaus, B., A. B\"{u}cher, and S. Volgushev (2017).
		%BETINA BERGHAUS*, AXEL BÜCHER** and STANISLAV VOLGUSHEV
		\newblock  Weak convergence of the empirical copula process with respect to weighted metrics.
\newblock {\em  Bernoulli\/} {\em 23}, 743--772. \doi{10.3150/15-BEJ751}

					      %\bibitem[\protect\citeauthoryear{Bradley}{Bradley}{2005}]{brad05}
        %Bradley, R.-C. (2005).
     %\newblock Basic properties of strong mixing conditions. A survey and some open questions.
     %\newblock {\em Probability Surveys\/} {\em 2}, 107--144. \doi{10.1214/154957805100000104}
											%\bibitem[\protect\citeauthoryear{Bernanke \textit{et al.}}{Bernanke \textit{et al.}}{2005}]{bertal05}
		%Bernanke, B.~S., J. Boivin, P. Eliasz (2005).
		%\newblock  Measuring the effects of monetary policy: a factor-augmented vector autoregressive (FAVAR) approach.
%\newblock {\em The Quarterly Journal of Economics\/} {\em 120}, 387--422. \doi{10.1162/0033553053327452}
%
		%%
									%\bibitem[\protect\citeauthoryear{Boivin \textit{et al.}}{Boivin \textit{et al.}}{2009}]{boetal09}
		%Boivin, J., M.~P. Giannoni, and I. Mihov (2009).
		%\newblock  Sticky prices and monetary policy: evidence from disaggregated US data.
%\newblock {\em American Economic Review\/} {\em 99}, 350--384. \doi{10.1257/aer.99.1.350}
		%
%
      %\bibitem[\protect\citeauthoryear{Bollerslev \textit{et al.}}{Bollerslev \textit{et al.}}{1994}]{boletal94}
        %Bollerslev, T., R.~F. Engle, and D.~B. Nelson (1994).
     %\newblock {\em ARCH Model.\/} in: Engle, R. F.,  and D. McFadden (Eds.), Handbook of Econometrics, {\em 4}, Amsterdam: North-Holland.
		%
							%\bibitem[\protect\citeauthoryear{Brown and Wegkamp}{Brown and Wegkamp}{2002}]{brwe02}
		%Brown, D.~J., and M.~H. Wegkamp (2002).
		%\newblock  Weighted minimum mean–square distance from independence estimation.
%\newblock {\em Econometrica\/} {\em 70}, 2035--2051. \doi{10.1111/1468-0262.00362}

					\bibitem[\protect\citeauthoryear{B\"{u}cher and Volgushev}{B\"{u}cher and Volgushev}{2013}]{buvo13}
		B\"{u}cher, A., and S. Volgushev (2013).
		\newblock  Empirical and sequential empirical copula processes under serial dependence.
\newblock {\em Journal of Multivariate Analysis\/} {\em 119}, 61--70. \doi{10.1016/j.jmva.2013.04.003}
 

					\bibitem[\protect\citeauthoryear{B\"{u}cher and Segers}{B\"{u}cher and Segers}{2013}]{buse13}
		B\"{u}cher, A., and J. Segers (2013).
		\newblock  Extreme value copula estimation based on block maxima of a multivariate stationary time series.
\newblock {\em Extremes\/} {\em 17}, 495--528. \doi{10.1007/s10687-014-0195-8}


					%\bibitem[\protect\citeauthoryear{Caporale \textit{et al.}}{Caporale \textit{et al.}}{2005}]{carpetal07}
		%Caporale, G.~M., C., Ntantamis, T., Pantelidis, and N. Pittis (2007).
		%%BETINA BERGHAUS*, AXEL BÜCHER** and STANISLAV VOLGUSHEV
		%\newblock  The BDS Test as a Test for the Adequacy of a GARCH(1,1) Specification: A Monte Carlo Study.
%\newblock {\em  Journal of Financial Econometrics\/} {\em 3}, 282--309. \doi{10.1093/jjfinec/nbi010}
%
%
%
			%\bibitem[\protect\citeauthoryear{Chen \textit{et al.}}{Chen \textit{et al.}}{2003}]{chetal03}
		%Chen, X., O. Linton, and I. Van Keilegom (2003).
		%\newblock Estimation of semiparametric models when the criterion function is not smooth.
%\newblock {\em Econometrica\/} {\em 71}, 1591--1608. \doi{10.1111/1468-0262.00461}


					%\bibitem[\protect\citeauthoryear{Chen and Fan}{Chen and Fan}{2006}]{chef06}
		%Chen, X., and Y. Fan (2006).
		%\newblock Estimation and model selection of semiparametric copula-based multivariate dynamic models under copula misspecification.
%\newblock {\em Journal of Econometrics\/} {\em 135}, 125--154. \doi{10.1016/j.jeconom.2005.07.027}
%
%%
			%\bibitem[\protect\citeauthoryear{Chen \textit{et al.}}{Chen \textit{et al.}}{2020}]{chetal20}
		%Chen, X., Z. Huang, and Y. Yi (2020).
		%\newblock
%Efficient estimation of multivariate semi-nonparametric GARCH filtered copula models.
%\newblock {\em Journal of Econometrics\/}. \doi{10.1016/j.jeconom.2020.07.012}
%
			%\bibitem[\protect\citeauthoryear{Cheng}{Cheng}{2015}]{cheng15}
		%Cheng, G. (2015).
		%\newblock
%Moment consistency of the exchangeably weighted bootstrap for semiparametric M-estimation.
%\newblock {\em Scandinavian Journal of Statistics\/}. {\em 42}, 665--684. \doi{10.1111/sjos.12128}
%
					%\bibitem[\protect\citeauthoryear{C\^{o}t\'{e} \textit{et al.}}{C\^{o}t\'{e} \textit{et al.}}{2019}]{cotetal19}
		%C\^{o}t\'{e}, M.-P., C. Genest, and M. Omelka (2019).
		%\newblock Rank-based inference tools for copula regression, with property and casualty insurance applications.
%\newblock {\em  Insurance: Mathematics and Economics\/} {\em 89}, 1--15.  \doi{j.insmatheco.2019.08.001}
%
					%\bibitem[\protect\citeauthoryear{Creal \textit{et al.}}{Creal \textit{et al.}}{2013}]{cretal13}
		%Creal, D.~D., S.~J. Koopman, and A. Lucas (2013).
		%\newblock Generalized autoregressive score models with applications.
%\newblock {\em Journal of Applied Econometrics\/} {\em 28}, 777--795. \doi{10.1002/jae.1279}
%
					%\bibitem[\protect\citeauthoryear{Creal and Tsay}{Creal and Tsay}{2015}]{crts15}
		%Creal, D.~D., and R.~S. Tsay (2015).
		%\newblock High dimensional dynamic stochastic copula models.
%\newblock {\em Journal of Econometrics\/} {\em 189}, 335-345. \doi{10.1016/j.jeconom.2015.03.027}



				%\bibitem[\protect\citeauthoryear{D'Errico}{D'Errico}{2021}]{derr21}
		%D'Errico, J. (2021).
		%\newblock fminsearchbnd, fminsearchcon.
%\newblock {\em MATLAB Central File Exchange\/} Retrieved April 17, 2021.
 %
				%\bibitem[\protect\citeauthoryear{Dette \textit{et al.}}{Dette \textit{et al.}}{2009}]{detal09}
		%Dette, H., J.~C. Pardo-Fern\'{a}ndez, and V.~I. Keilegom (2009).
		%\newblock Goodness-of-fit tests for multiplicative models with dependent data.
%\newblock {\em Scandinavian Journal of Statistics\/} {\em 36}, 782--799. \doi{110.1111/j.1467-9469.2009.00648.x}

					%\bibitem[\protect\citeauthoryear{De Lira Salvatierra and Patton}{De Lira Salvatierra and Patton}{2015}]{dlspa15}
		%De Lira Salvatierra, I., and A.~J. Patton (2015).
		%\newblock Dynamic copula models and high frequency data.
%\newblock {\em Journal of Empirical Finance\/} {\em 30}, 120--135. \doi{10.1016/j.jempfin.2014.11.008}
%

					%\bibitem[\protect\citeauthoryear{Doukhan \textit{et al.}}{Doukhan \textit{et al.}}{1995}]{dotal95}
		%Doukhan, P., P. Massart, and E. Rio (1995).
		%\newblock Invariance principles for absolutely regular empirical processes.
%\newblock {\em Annales de l'I.H.P--Probabilit\'{e}s et statistiques\/} {\em 31}, 393--427. 

					%\bibitem[\protect\citeauthoryear{Duan \textit{et al.}}{Duan \textit{et al.}}{2019}]{dutal19}
		%Duan, F., H. Manner, and D. Wied (2019).
		%\newblock  Model and moment selection in factor copula models.
%\newblock {\em Journal of Financial Econometrics\/} {\em 39}, 1--31. \doi{10.1093/jjfinec/nbz039}

					%\bibitem[\protect\citeauthoryear{Escanciano \textit{et al.}}{Escanciano \textit{et al.}}{2018}]{escal18}
		%Escanciano, J.~C., J.~C. Pardo-Fern\'{a}ndez, and I. Van Keilegom (2018).
		%\newblock Asymptotic distribution-free tests for semiparametric regressions with dependent data.
%\newblock {\em Annals of Statistics\/} {\em 46}, 1167--1196. \doi{10.1214/17-AOS1581}


					\bibitem[\protect\citeauthoryear{Fantazzini}{Fantazzini}{2008}]{fanta08}
		Fermanian, D. (2008).
		\newblock  Dynamic copula modelling for value at risk.
\newblock {\em Frontiers in Finance and Economics\/} {\em 5}, 72--108. \doi{10.3150/bj/1099579158}


      %\bibitem[\protect\citeauthoryear{Fan and Patton}{Fan and Patton}{2014}]{fapa14}
        %Fan, Y., and A.~J. Patton (2014).
		%\newblock Copulas in econometrics.
%\newblock {\em Annual Review of Economics\/} {\em 6}, 179--200. \doi{10.1146/annurev-economics-080213-041221}
		
					\bibitem[\protect\citeauthoryear{Fermanian \textit{et al.}}{Fermanian \textit{et al.}}{2004}]{fetal04}
		Fermanian, J.-D., D. Radulovi\'{c}, and M.~H. Wegkamp (2004).
		\newblock  Weak convergence of empirical copula processes.
\newblock {\em  Bernoulli\/} {\em 10}, 847--860. \doi{10.3150/bj/1099579158}


					%\bibitem[\protect\citeauthoryear{Fermanian and Wegkamp}{Fermanian and Wegkamp}{2012}]{fewe12}
		%Fermanian, J.-D., and M.~H. Wegkamp (2012).
		%\newblock  Time-dependent copulas.
%\newblock {\em  Journal of Multivariate Analysis} {\em 110}, 19--29. \doi{10.1016/j.jmva.2012.02.018}

					%\bibitem[\protect\citeauthoryear{Francq and Zako\"ian}{Francq and Zako\"ian}{2004}]{fraz04}
		%Francq, C., and J.-M. Zako\"ian (2004).
		%\newblock   Maximum likelihood estimation of pure GARCH and ARMA-GARCH processes.
%\newblock {\em  Bernoulli} {\em 4}, 605--637. \doi{10.3150/bj/1093265632}
					%\bibitem[\protect\citeauthoryear{Genest \textit{et al.}}{Genest \textit{et al.}}{2007}]{genestetal07}
		%Genest, C., K. Ghoudi, and B. R\'{e}millard (2007).
		%\newblock  Rank-Based Extensions of the Brock, Dechert, and Scheinkman Test.
%\newblock {\em  Journal of the American Statistical Association\/} {\em 102}, 1363--1376. \doi{10.1198/016214507000001076}

					%\bibitem[\protect\citeauthoryear{Gijbels \textit{et al.}}{Gijbels \textit{et al.}}{2015}]{gibetal15}
		%Gijbels, I., M. Omelka, and  N. Veraverbeke  (2015).
		%\newblock  Estimation of a copula when a covariate affects only marginal distributions.
%\newblock {\em Scandinavian Journal of Statistics\/} {\em 42}, 1109--1126. \doi{10.1111/sjos.12154}

					%\bibitem[\protect\citeauthoryear{Gijbels \textit{et al.}}{Gijbels \textit{et al.}}{2017}]{gibetal17}
		%Gijbels, I., M. Omelka, M. Pe$\check{\textnormal{s}}$ta, and  N. Veraverbeke  (2017).
		%\newblock Score tests for covariate effects in conditional copulas.
%\newblock {\em Journal of Multivariate Analysis\/} {\em 159}, 111--133. \doi{10.1016/j.jmva.2017.05.001}

			%\bibitem[\protect\citeauthoryear{Gin\'{e} and Zinn}{Gin\'{e} and Zinn}{1990}]{gizi90}
		%Gin\'{e}, E., and J. Zinn (1990).
		%\newblock   Bootstrapping general empirical measures.
%\newblock {\em  Annals of Probability} {\em 18}, 851–869. \doi{10.1214/aop/1176990862}

%GINÉ, E., AND J. ZINN (1990): "Bootstrapping General EmpiricalMeasures," Annals of Probability,
%18, 851–869.

					%\bibitem[\protect\citeauthoryear{Goncalves and White}{Goncalves and White}{2004}]{gowi04}
		%Gonçalves, S., and H. White (2004).
		%\newblock Maximum likelihood and the bootstrap for nonlinear dynamic models.
%\newblock {\em Journal of Econometrics\/} {\em 119}, 199--219. \doi{10.1016/S0304-4076(03)00204-5}


					%\bibitem[\protect\citeauthoryear{Gon\c{c}alves \textit{et al.}}{Gon\c{c}alves \textit{et al.}}{2019}]{gonetal19}
		%Gon\c{c}alves, S., U. Hounyo, A.~J. Patton, and K. Sheppard (2019).
		%\newblock Bootstrapping two-stage quasi-maximum likelihood estimators of time series models.
%\newblock {\em Working paper\/}
%
%
%\bibitem[\protect\citeauthoryear{Gouri\'{e}roux  and Monfort}{Gouri\'{e}roux  and Monfort}{1997}]{gofo97}
        %Gouri\'{e}roux, C., and A. Monfort (1997).
     %\newblock {\em Simulation-based Econometric Methods.\/} CORE Lectures.
     %\newblock Oxford: Oxford University Press.
%
					%\bibitem[\protect\citeauthoryear{Hansen}{Hansen}{1994}]{hansen94}
		%Hansen, B. (1994).
		%\newblock Autoregressive conditional densityestimation.
%\newblock {\em International Economic Review\/} {\em 35}, 705--730. \doi{10.2307/2527081.}
%
					%\bibitem[\protect\citeauthoryear{Hong \textit{et al.}}{Hong \textit{et al.}}{2021}]{hongetal21}
		%Hong, H., H. Li, and J. Li, (2021).
		%\newblock BLP estimation using Laplace transformation and overlapping simulation draws.
%\newblock {\em Journal of Econometrics\/} {\em 222}, 56--72. \doi{10.1016/j.jeconom.2020.07.026.}

						\bibitem[\protect\citeauthoryear{Kosorok}{Kosorok}{2008}]{ko08}
	Kosorok, M.~R.  (2008). 
		 \newblock {\em Introduction to Empirical Processes and Semiparametric Inference\/},
		 \newblock Springer Series in Statistics, Berlin: Springer.

					%\bibitem[\protect\citeauthoryear{Krupskii and Joe}{Krupskii and Joe}{2013}]{kj13}
		%Krupskii, P. and H. Joe (2013).
		%\newblock Factor copula models for multivariate data.
%\newblock {\em Journal of Multivariate Analysis\/} {\em 120}, 85--101. \doi{10.1016/j.jmva.2013.05.001.}
%
					%\bibitem[\protect\citeauthoryear{Krupskii and Joe}{Krupskii and Joe}{2020}]{kj20}
		%Krupskii, P. and H. Joe (2020).
		%\newblock Flexible copula models with dynamic dependence and application to financial data.
%\newblock {\em Econometrics and Statistics\/} {\em 16}, 148--167. \doi{10.1016/j.ecosta.2020.01.00.}


%
					%\bibitem[\protect\citeauthoryear{Lee}{Lee}{1992}]{lee92}
		 %Lee, J. F. (1992).
		%\newblock On efficiency of methods of simulated moments and maximum simulated likelihood estimation of discrete response models.
%\newblock {\em Econometric Theory\/} {\em 8}, 518--552. \doi{10.1017/S0266466600013207}

			%\bibitem[\protect\citeauthoryear{Lee}{Lee}{1995}]{lee95}
		 %Lee, J. F. (1995).
		%\newblock Asymptotic bias in simulated maximum likelihood estimation of discrete choice models.
%\newblock {\em Econometric Theory\/} {\em 11}, 437--483. \doi{10.1017/S0266466600009361}


	%\bibitem[\protect\citeauthoryear{Newey and McFadden}{Newey and McFadden}{1994}]{nemc94}
		 %Newey, W.~K., and D. McFadden (1994).
		%\newblock Large sample estimation and hypothesis testing, 
%\newblock {\em in Handbook of Econometrics\/} {\em 4}, ed by R. Engle and D. McFadden.  Amsterdam: North Holland, 2113--2247. \doi{10.1016/S1573-4412(05)80005-4}

					%\bibitem[\protect\citeauthoryear{Manner \textit{et al.}}{Manner \textit{et al.}}{2019}]{manetal19}
		%Manner, H., F. Stark, and D. Wied (2019).
		%\newblock Testing for structural breaks in factor copula models.
%\newblock {\em Journal of Econometrics\/} {\em  208}, 324--345.  \doi{10.1016/j.jeconom.2018.10.001.}
%
					%\bibitem[\protect\citeauthoryear{Manner \textit{et al.}}{Manner \textit{et al.}}{forthcoming}]{manetal20}
		%Manner, H., F. Stark, and D. Wied (forthcoming).
		%\newblock A monitoring procedure for detecting structural breaks in factor copula models.
%\newblock {\em Studies in Nonlinear Dynamics \& Econometrics\/} \doi{10.1515/snde-2019-0081.}




%\bibitem[\protect\citeauthoryear{McFadden}{McFadden}{1989}]{mcf89}
		 %McFadden, D. (1989).
		%\newblock A method of simulated moments for estimation of discrete response models without numerical integration.
%\newblock {\em Econometrica\/} {\em 57}, 995--1026. \doi{10.2307/1913621}
%
 							%%\bibitem[\protect\citeauthoryear{Neumeyer and Van Keilegom}{Neumeyer and Van Keilegom}{2010}]{neukeil10}
		%Neumeyer, N.,  and I.~Van Keilegom (2019).
		%\newblock  Estimating the error distribution in nonparametric multiple regression with applications to model testing.
%\newblock {\em  Journal of Multivariate Analysis\/} {\em 101}, 1067--1078. \doi{10.1016/j.jmva.2010.01.007}

 							\bibitem[\protect\citeauthoryear{Neumeyer \textit{et al.}}{Neumeyer \textit{et al.}}{2019}]{neumetal19}
		Neumeyer, N., M. Omelka, and $\check{\textnormal{S}}$. Hudecov\'{a} (2019).
		\newblock  A copula approach for dependence modeling in multivariate nonparametric time series.
\newblock {\em  Journal of Multivariate Analysis\/} {\em 171}, 139--162. \doi{10.1016/j.jmva.2018.11.016}




%\bibitem[\protect\citeauthoryear{Newey}{Newey}{1994}]{new94}
		 %Newey, K. W. (1994).
		%\newblock The asymptotic variance of semiparametric estimators.
%\newblock {\em Econometrica\/} {\em 62}, 1349--1382. %\doi{10.3390/econometrics5010013}


					%\bibitem[\protect\citeauthoryear{Oh and Patton}{Oh and Patton}{2013}]{ohpa13}
		 %Oh, D.~H., and A.~J. Patton (2013).
		%\newblock Simulated method of moments estimation for copula-based multivariate models.
%\newblock {\em Journal of the American Statistical Association\/} {\em 108}, 689--700. \doi{10.1080/01621459.2013.785952}
%
%
					%\bibitem[\protect\citeauthoryear{Oh and Patton}{Oh and Patton}{2017}]{ohpa17}
		 %Oh, D.~H., and A.~J. Patton (2017).
		%\newblock Modeling dependence in high dimensions with factor copulas.
%\newblock {\em Journal of Business \& Economic Statistics\/} {\em 35}, 139--154. \doi{10.1080/07350015.2015.1062384}
%
					%\bibitem[\protect\citeauthoryear{Oh and Patton}{Oh and Patton}{2018}]{ohpa18}
		 %Oh, D.~H., and A.~J. Patton (2018).
		%\newblock Time-varying systemic risk: evidence from a dynamic copula model of CDS spreads.
%\newblock {\em Journal of Business \& Economic Statistics\/} {\em 36}, 181--195. \doi{10.1080/07350015.2016.1177535}
%
%
					%\bibitem[\protect\citeauthoryear{Oh and Patton}{Oh and Patton}{2021}]{ohpa21}
		 %Oh, D.~H., and A.~J. Patton (2021).
		%\newblock  Factor copula models with estimated cluster assignments.
%\newblock {\em Finance and Economics Discussion Series\/} {\em 2021-029},  Washington: Board of Governors of the Federal Reserve System. \doi{doi.org/10.17016/FEDS.2021.029}
%

%
					%\bibitem[\protect\citeauthoryear{Omelka \textit{et al.}}{Omelka \textit{et al.}}{2020}]{ometal20}
		%Omelka, M., N. Neumeyer, and $\check{\textnormal{S}}$. Hudecov\'{a} (2020).
		%\newblock  Maximum pseudo-likelihood estimation based on estimated residuals in copula semiparametric models.
%\newblock {\em  Scandinavian Journal of Statistics\/}, 1--41.  \doi{10.1111/sjos.12498}
%
					%\bibitem[\protect\citeauthoryear{Opschoor \textit{et al.}}{Opschoor \textit{et al.}}{2020}]{opetal20}
		  %Opschoor, A., Lucas, A, Barra, I., and van Dijk, D. (2020). 
		%\newblock Closed-form multi-factor copula models with observation-driven dynamic factor loadings.
%\newblock {\em Journal of Business \& Economic Statistics\/} \doi{10.1080/07350015.2020.1763806}
%
%
	%\bibitem[\protect\citeauthoryear{Pakes and Pollard}{Pakes and Pollard}{1989}]{papo89}
		 %Pakes, A., and D. Pollard (1989).
		%\newblock Simulation and the asymptotics of optimization estimators.
%\newblock {\em Econometrica\/} {\em 57}, 1027--1057. \doi{10.2307/1913622}

	%\bibitem[\protect\citeauthoryear{Patton}{Patton}{2006}]{pat06}
		 %Patton, A. (2006).
		%\newblock Modelling asymmetric exchange rate dependence.
%\newblock {\em International Economic Review\/} {\em 47}, 527--556. \doi{10.1111/j.1468-2354.2006.00387.x}

				\bibitem[\protect\citeauthoryear{ Radulovi\'{c} \textit{et al.}}{Radulovi\'{c} \textit{et al.}}{2017}]{radetal17}
		 Radulovi\'{c}, D., Wegkamp, M., and Y. Zhao (2017).
		\newblock Weak convergence of empirical copula processes indexed by functions.
\newblock {\em Bernoulli\/} {\em 23}, 3346--3384. \doi{10.3150/16-BEJ849}

				%\bibitem[\protect\citeauthoryear{R\'{e}millard}{R\'{e}millard}{2017}]{rem17}
		 %R\'{e}millard, B. (2017).
		%\newblock Goodness-of-fit tests for copulas of multivariate time series.
%\newblock {\em econometrics\/} {\em 5}, 1--23. \doi{10.3390/econometrics5010013}

					\bibitem[\protect\citeauthoryear{Resnick}{Resnick}{1999}]{res99}
		Resnick, S.  (1999). \newblock {\em  A Probability Path. \/} World Publishing Corporation.


\bibitem[\protect\citeauthoryear{Shaw}{Shaw}{2006}]{shaw06}
		Shaw, W. (2006).
		\newblock Sampling Student's \(T\) distribution--use of the inverse cumulative distribution function.
\newblock {\em The Journal of Computational Finance\/} {\em 9}, 37--73. \doi{10.21314/JCF.2006.150}

					%\bibitem[\protect\citeauthoryear{Segers}{Segers}{2012}]{seg12}
		 %Segers, J. (2012).
		%\newblock Asymptotics of empirical copula processes under nonrestrictive smoothness assumptions.
%\newblock {\em Bernoulli\/} {\em 18}, 764--782. \doi{10.3150/11-BEJ387}

					%\bibitem[\protect\citeauthoryear{Stock and Watson}{Stock and Watson}{2005}]{stwa05}
		 %Stock, J.~H., and M.~W. Watson (2005).
		%\newblock Implications of dynamic factor models for VAR analysis.
%\newblock {\em NBER Working Paper\/} {\em 11467}. \doi{10.3386/w11467}


					%\bibitem[\protect\citeauthoryear{Tsukahara}{Tsukahara}{2005}]{tak05}
		 %Tsukahara, H. (2005).
		%\newblock Semiparametric estimation in copula models. 
%\newblock {\em Canadian Journal of Statistics\/} {\em 33}, 357--375. \doi{10.1002/cjs.5540330304}


						\bibitem[\protect\citeauthoryear{van der Vaart}{van der Vaart}{1994}]{vv94}
	van der Vaart, A.~W.  (1994). 
		 \newblock {\em Asymptotic Statistics\/},
		 \newblock Cambridge Series in Statistical and Probabilistic Mathematics, Cambridge: Cambridge University Press.
		
      \bibitem[\protect\citeauthoryear{van der Vaart and Wellner}{van der Vaart and Wellner}{1996}]{vw96}
        van der Vaart, A. W., and J.~A. Wellner (1996).
     \newblock {\em Weak convergence and empirical processes.\/}
     \newblock New York: Springer.
 
      %\bibitem[\protect\citeauthoryear{van der Vaart and Wellner}{van der Vaart and Wellner}{2007}]{vw07}
        %van der Vaart, A. W., and J.~A. Wellner (2007).
     %\newblock {\em Empirical processes indexed by estimated functions.\/} in: E.~A. Cator, G.~Jongbloed, C.~Kraaikamp, H.~P. Lopuha\"{a}, J.~A. Wellner (Eds.), Asymptotics: Particles, Processes and Inverse Problems, Hayward: Institute of Mathematical Statistics.

										\bibitem[\protect\citeauthoryear{White}{White}{2001}]{white01}
		White, H.  (2001). 
		 \newblock {\em Asymptotic Theory for Econometricians\/},
		 \newblock 2nd ed., Bingley: Emerald.
