# Supplementary material for: Estimation and Inference in Factor Copula Models with Exogenous Covariates
Source: arXiv:2107.03366 source file (2022-12-01)
Supplement: Supplementary file 2 [file online_supplement.tex]

\input{preamble}
\usepackage{lineno}
\usepackage[affil-it]{authblk}
 \usepackage{xr-hyper}

\renewcommand{\thesection}{S.\arabic{section}}
\renewcommand{\theequation}{S.\arabic{equation}}
\renewcommand{\thetheorem}{S\arabic{theorem}}
\renewcommand{\theassumption}{S.\arabic{assumption}}
\renewcommand{\theproposition}{S.\arabic{proposition}}
\renewcommand{\thecorollary}{S.\arabic{corollary}}
\renewcommand{\thelemma}{S.\arabic{lemma}}
\renewcommand{\theexample}{S.\arabic{example}}
\renewcommand{\theremark}{S.\arabic{remark}}
%\newcommand*{\at}[2][]{#1|_{#2}} 
 
 \title{Supplement to `Estimation and Inference in Factor Copula Models with Exogenous Covariates'}
\author[1,a]{Alexander Mayer}
\author[2]{Dominik Wied\vspace*{-.5cm}}
\affil[1]{%
Department of Economics, Universit\`{a} Ca' Foscari Venezia}
\affil[2]{%
   Institute of Econometrics and Statistics, University of Cologne} 
\affil[a]{\small \textnormal{Corresponding author, email: \href{mailto:alexandersimon.mayer@unive.it}{alexandersimon.mayer@unive.it}}}
	\date{\today}

%\author{First Last%
  
\externaldocument[]{master}
\begin{document}
\maketitle 
\linenumbers
%\section{Proof of lemma \ref{lemmaV}, \ref{lemmaU}, and \ref{lemmaA3}}
\input{online_supplementbody}

%
%\newpage
\addcontentsline{toc}{section}{References}
\begin{thebibliography}{}
\input{copula_ref_supp}
\end{thebibliography}{}
\end{document}
